# Supplementary material for: Conservation and losses of avian non-coding RNA loci
Source: arXiv:1406.7140 source file (2014-06-27)
Supplement: Supplementary file 1 [file supplementary-material.pdf]

# Supplementary material for: non-coding RNAs of bird genomes

Paul P. Gardner*[1,2] , Mario Fasold[5] , Sarah W. Burge[3] , Jana Hertel[5] , Maria Ninova[4] , Stephanie Kehr[5] , Tammy E. Steeves[1] , Sam Griffiths-Jones[4] and Peter Stadler*[5]

[1] School of Biological Sciences, University of Canterbury, Private Bag 4800, Christchurch, New Zealand. [2] Biomolecular Interaction Centre, University of Canterbury, Private Bag 4800, Christchurch, New Zealand. [3] European Molecular Biology Laboratory, European Bioinformatics Institute, Hinxton, Cambridge, CB10 1SD, UK. [4] Faculty of Life Sciences, University of Manchester, Manchester, United Kingdom. [5] Bioinformatics Group, Department of Computer Science; and Interdisciplinary Center for Bioinformatics, University of Leipzig, Härtelstrasse 16-18, D-04107 Leipzig, Germany

Email: Paul P. Gardner*- paul.gardner@canterbury.ac.nz; mario@bierdepot.bioinf.uni-leipzig.de; sb30@sanger.ac.uk; Jana Hertel*- jana@bioinf.uni-leipzig.de; Maria.Ninova@postgrad.manchester.ac.uk; steffi@bierdepot.bioinf.uni-leipzig.de; tammy.steeves@canterbury.ac.nz; sam.griffiths-jones@manchester.ac.uk; Peter Stadler*- studla@bioinf.uni-leipzig.de;

*To whom correspondence should be addressed

## Supplementary results

In the following we explore in further detail the results that were not discussed in the main manuscript.

### Classic RNAs: LUCA and LECA

Many RNA families constitute the most evolutionarily conserved genes across all life on this planet [1]. Examples of RNAs derived from the Last Universal Common Ancestor (LUCA) include, the transfer RNAs (tRNA), ribosomal RNAs (rRNA), RNA components of RNase P (RNase P RNA), RNase MRP (RNase MRP RNA) and the signal recognition particle (SRP RNA). Other classes of RNA are likely to have been components of the Last Eukaryotic Common Ancestor (LECA) include the telomerase RNA, major spliceosomal RNAs (U1, U2, U4, U5, and U6) and the minor spliceosomal RNAs (U11, U12, U4atac, and U6atac) [2].

Unsurprisingly, the bulk of these classes of RNAs are well represented across the bird genomes (See Figure 2). However, there appear to have been "losses" of a few of these RNAs in certain bird species. Some of these may be due to sequence divergence, of which there are several notable examples e.g. [3–7]. Other losses may be due to incomplete genome coverage.

A number of the classic RNAs are incorporated into RNA-protein complexes (RNPs) involved in core

cellular processes. An example of this are the spliceosomal RNAs. Based upon the presence/absence patterns of the major spliceosomal RNAs they are all well represented in these genome sequences. The exceptions to this observation are the U4 RNA in cormorant and the U5 RNA in the bee eater which are both missing. These two genomes are low coverage, suggesting these genes weren't captured in the current assembly. The minor spliceosomal RNAs are more interesting, the U4atac and U11 snRNAs show widespread patterns of loss, even in some of the high coverage genomes. These RNAs are frequently missed in bioinformatic screens. Indicating either frequent loss [8] or sequences that have diverged beyond the ability of detection by covariance models [9].

The telomerase RNA is also largely missing from the avian annotations. This RNA acts as a template for the telomerase enzyme that extends the telomeres found on chromosome ends. It is only found in the chicken, bald eagle, kea, budgerigar, crow and zebrafinch. Homology searches searches with the telomerase reverse transcriptase (TERT) protein show that the protein component of the telomerase RNP is conserved across all the bird genomes (data not shown). This pattern of presumably divergent telomerase RNA and conserved telomerase protein has been noted previously, most notably in the fungi [3, 4].

The RNA components of RNase P and RNase MRP also appear to have undergone dramatic losses within the bird lineage. RNase P is required for the maturation of tRNA, the paralogous enzyme, RNase MRP is required for the maturation of rRNA. Each RNP cleaves smaller RNAs from larger transcripts [10]. It is unlikely that the these genes have been lost in any of the birds. Homology searches with the RNase associated protein coding genes (POP1, POP4, POP5, POP7, RPP1, RPP14, RPP25, RPP38, RPP40 and RPR2), identified viable homologs of each in all of the bird genomes [11] (data not shown). This suggests that the bird RNase P and MRP RNAs may have diverged slightly from the canonical models.

The 5.8 S component of the ribosome in the turtle, turkey bustard, hoatzin, flamingo, tropicbird, seriema, owl, cuckoo roller, trogon, bee eater and falcon appears to have been lost (See Figure 2). The rRNA repeats are frequently not assembled, consequently it is not surprising to see "losses" in these [12]. Furthermore, the genomes for these species are also low-coverage.

### Small nucleolar RNAs

Small nucleolar RNAs (snoRNAs) are important ncRNAs that participate in the maturation of other functional RNAs [13]. The bulk of the characterised snoRNAs guide either methylation or pseudouridylation modifications, primarily of rRNAs but also spliceosomal RNAs. The two types of modifications are guided by two different types of RNA, the box C/D and the H/ACA snoRNAs

respectively, each with a characteristic cohort of motifs and secondary structures [14].

There are 66 ribosomal modification sites, guided by 59 snoRNA families, that are preserved between *H. sapiens* and *S. cerevisiae* [15]. Of these, 45 snoRNA families are conserved in the bird data set. Over a third of the apparent losses of the yeast-human conserved snoRNA families appear to cluster on 2 loci of the ancestral vertebrate genome. We investigated these losses further.

The first cluster is found at chr11:62620797-62622484 on the human genome (hg19) and contains SNORD27, SNORD29 and SNORD31 of the human-yeast conserved snoRNAs. These snoRNAs are located in the inside-out gene SNHG1 which hosts a total of eight C/D box snoRNAs: SNORD25, SNORD26, SNORD27, SNORD28, SNORD29, SNORD22, SNORD30 and SNORD31 [16]. Each of which are also found in the alligator and turtle genomes within a 3-4 KB locus, yet these have largely been lost in the birds. However, five of the eight snoRNAs are located in the tinamou genome. These are located on the same scaffold and are within 2 KB of each other. This implies that SNHG1 is conserved in the tinamou. Loci with four of the eight snoRNAs can be found in zebrafinch, ground-finch, and bald eagle. Still, three of the eight are located in the ostrich, crow, and cuckoo genomes, again within 2 KB of each other on the same scaffolds. This complex pattern of loss could be attributed to many different models, e.g. multiple losses in birds, poor homology modelling or incomplete genome sequences.

The second cluster is located at chr19:49993222-49994231 on the human genome (hg19) and contains two copies of SNORD33 and one SNORD34 all within a 1 KB genomic region. The turtle and alligator genomes retain the two copies of SNORD33 yet don't have an obvious SNORD34 gene on the same scaffold. Within the bird genomes, the crow and rifleman each retain a single SNORD33 and SNORD34 gene on the same scaffold. While the ground-finch and bald eagle retain a single SNORD33 and the zebrafinch and seriema retain a single SNORD34 (See Supplemental Figure 3). In human these snoRNAs are intronic to the host gene, ribosomal protein L13a (RPL13A). Based on BLASTP (version 2.2.18) homology searches for the RPL13A gene, the protein is conserved in the human and turtle genomes and in the bald eagle, crow, rifleman and zebrafinch avian genomes (data not shown). Therefore the RPL13A gene and corresponding intronic snoRNAs show the same conservation pattern. This supports a pattern of loss of the RPL13A gene and the intronic snoRNAs that it hosts in the bird genomes.

### MicroRNAs

MicroRNAs are an important class of non-coding RNA. They have been found in the genomes of Chromalveolata [17,18], Metazoa [19–21], Mycetozoa [22,23], Viridiplantae [24–27] and Viruses [28–31].

The miRNAs have been shown to regulate the expression of large numbers of messenger RNAs [32]. The mature miRNA product is generally 22 nucleotides long which is usually processed from a larger RNA that is characterised by a stable hairpin-shaped secondary structure.

Chicken and zebrafinch are the only birds with previously annotated microRNAs. We searched for homologs of these and other vertebrate microRNAs in the genomes of the 48 birds, American alligator and green turtle. Overall, we annotate a total of 16617 putative microRNA loci, homologous to 543 known microRNA genes, of which 487 are annotated in chicken and/or zebra finch, while 56 have been so far known only in non-avian vertebrates. The numbers of annotated loci in the individual species are approximately equal - 300-400 per species, except for the turkey (Meleagris gallopavo) where we identified 543 sequences homologous to known microRNAs.

In addition, we can confidently identify a further 3 microRNA families that are present in mammals, and turtle and/or crocodile, but not in any avian genome (mir-150, mir-208, mir-590). This suggests that these sequences were lost in the last common ancestor of archosaurs or birds. There are also a number of microRNAs that are predicted to be present in turtles and/or crocodiles, and only a small number of bird genomes. Indeed, there are many missing annotations, species-specific and otherwise, that are not consistent with the consensus phylogeny, and could be due to either incomplete genomes or widespread microRNA loss.

The turkey genome contains a high number (190) of microRNAs so far found only in chicken, which account for the higher number of annotated sequences in this genome compared with other birds. This is consistent with its phylogenetic position as the closest chicken relative among the examined birds. However, 101 chicken microRNAs have no homolog in the turkey or other bird genomes, suggesting that these genes are chicken-specific. This is consistent with previous reports of large number of species specific microRNAs in all animals, and supports the view of fast microRNA turnover during animal evolution.

### Cis-regulatory elements

The cis-regulatory RNAs are a group of RNA structures encoded on mRNAs. Generally they are involved in regulating the expression of the mRNA they are encoded within. Others may recode the translated protein product into an alternate sequence.

This group includes the iron response element (IRE) [33] and the histone $3'$ UTR (histone3) [34]. These are structured motifs bound by regulatory proteins. The selenocysteine insertion sequence (SECIS) is a structured motif that recodes UGA stop codons to selenocysteines [35] and the GABRA3 stem-loop is a

structure recognised by the ADAR enzyme family. This enzyme edits adenine nucleotides to inosine, in this case recoding an isoleucine codon to methionine in exon 9 of the GABRA3 gene [36].

These regulatory elements and others, including an internal ribosome entry site (IRES), potassium channel RNA editing signal (K chan RES), Antizyme RNA frameshifting stimulation element (Antizyme FSE), vimentin 3′ UTR protein-binding region (Vimentin3) and a connective tissue growth factor (CTGF) 3′ UTR element (CAESAR) are conserved across a diverse group of vertebrates, including the bird lineages explored here (See Figure 2).

### Unexpectedly poorly conserved ncRNAs: testing divergence

In order to get an idea to what extent the absence of these RNAs from the `infernal-based` annotation is caused by sequence divergence beyond the thresholds of the Rfam CMs and/or missing or incomplete data, we complemented our analysis by dedicated searches for a few of these RNA groups.

The simplest case are the selenocysteine tRNAs. Here, tRNAscan is tuned for specificity and thus misses several occurrences that are easily found by `blastn` with $E \leq 10^{-30}$. In some cases the sequences appear degraded at the ends, which may be explained e.g. by low sequence quality at the very ends of contigs or scaffolds. A `blastn` search also readily retrieves additional RNase P and RNAse MRP RNAs, capturing only the best conserved regions. In many cases these additional candidates are incomplete or contain undetermined sequence, explaining why they are missed by the CMs. Overall, we identify tRNA-Sec in most and RNAse P and MRP RNAs in the majority of the genomes. An additional candidate could also be retrieved for telomerase RNA. Telomerase is well known to exhibit very poor sequence conservation and rapid variations in size that make it notoriously hard to identify by homology search [37]. The poor return thus does not come as a surprise. Vault RNA homology searches with `blastn` remained unsuccessful, therefore we constructed a sauropsid-specific CM. In addition to the hits identified by the Rfam model we obtained three additional homologs. Vault RNAs, with a size of about 100 nt, exhibit conserved sequence patterns only at their ends, with essentially unconstrained sequence in the central part. Their identification is one of the well-known and difficult problems for homology search [38, 39].

Our ability to find additional homologs for several RNA families that fill gaps in the abundance matrices (Figure 1) strongly suggests that conspicuous absences, in particular of LUCA and LECA RNAs, are caused by incomplete data in the current assemblies and sequence divergence rather then true losses.

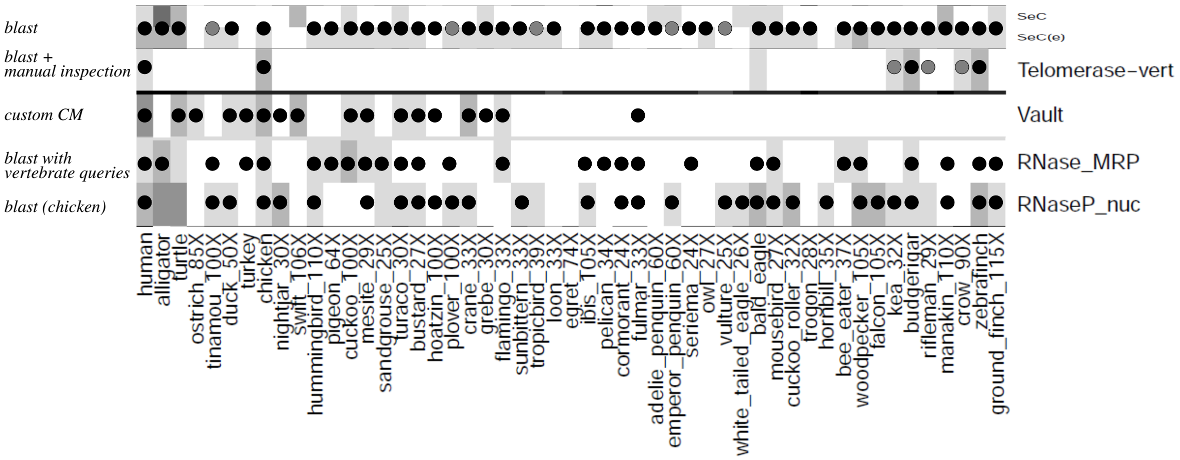


Figure 1: Additional homologs of some sparsely represented RNA families were discovered using dedicated search strategies combined with highly sensitive settings, synteny information, lineage-specific CMs and subsequent manual inspection.

### Exceptional RNAs

A number of other ncRNAs can also be found in Eukaryotic genomes. These do not fit into the main classes of RNA but still perform vital roles in the function and evolution of Eukaryotes. Their functions are diverse and many have not yet been characterised.

An example of an uncharacterised RNA is the ultraconserved element, uc.338 (also known as TUC338) [40–42]. The uc.338 element is derived from a short interspersed element (SINE) called the lobe-finned fishes SINE (LF-SINE) as it is conserved between the coelacanth and mammals [41]. Analysis of the expression of uc.338 implies that it plays a role in the progression of hepatocellular carcinoma, possibly by influencing cell growth [42]. This RNA is conserved in the birds and appears to have been duplicated in several lineages.

The Y RNA is an enigmatic ncRNA where we know very little about the function. It was discovered in the 1980s in ribonucleoprotein complexes [43]. The function of the Y RNAs remain unknown, but evidence is emerging that they may be associated with DNA replication [44]. There are 4 functional Y RNAs encoded in the human genome, Y1, Y3, Y4 and Y5. However, there are hundreds of pseudogenised copies of the Y RNA scattered throughout the human genome [45]. In the birds and other lizards, we identify between two and seven Y RNA paralogs (See Figure 2).

The Vault RNA forms a major component of the vault ribonucleoprotein complex, this is one of the largest particles found in the vertebrate cell; In fact, it is larger than the ribosome [46]. As yet not much is known

about the function of Vault. The Vault RNA has been shown to be broadly conserved in metazoans [47]. However, in the bird lineages it appears to have either been lost or diversified.

## Contamination

Bacterial families can be used to identify problematic sequences that are likely to be the result of contamination from non-avian sources. We identified a number of RNA families of bacterial origin in the avian genomes. These have been reported and will be dealt with in later updates to the avian genome sequences.

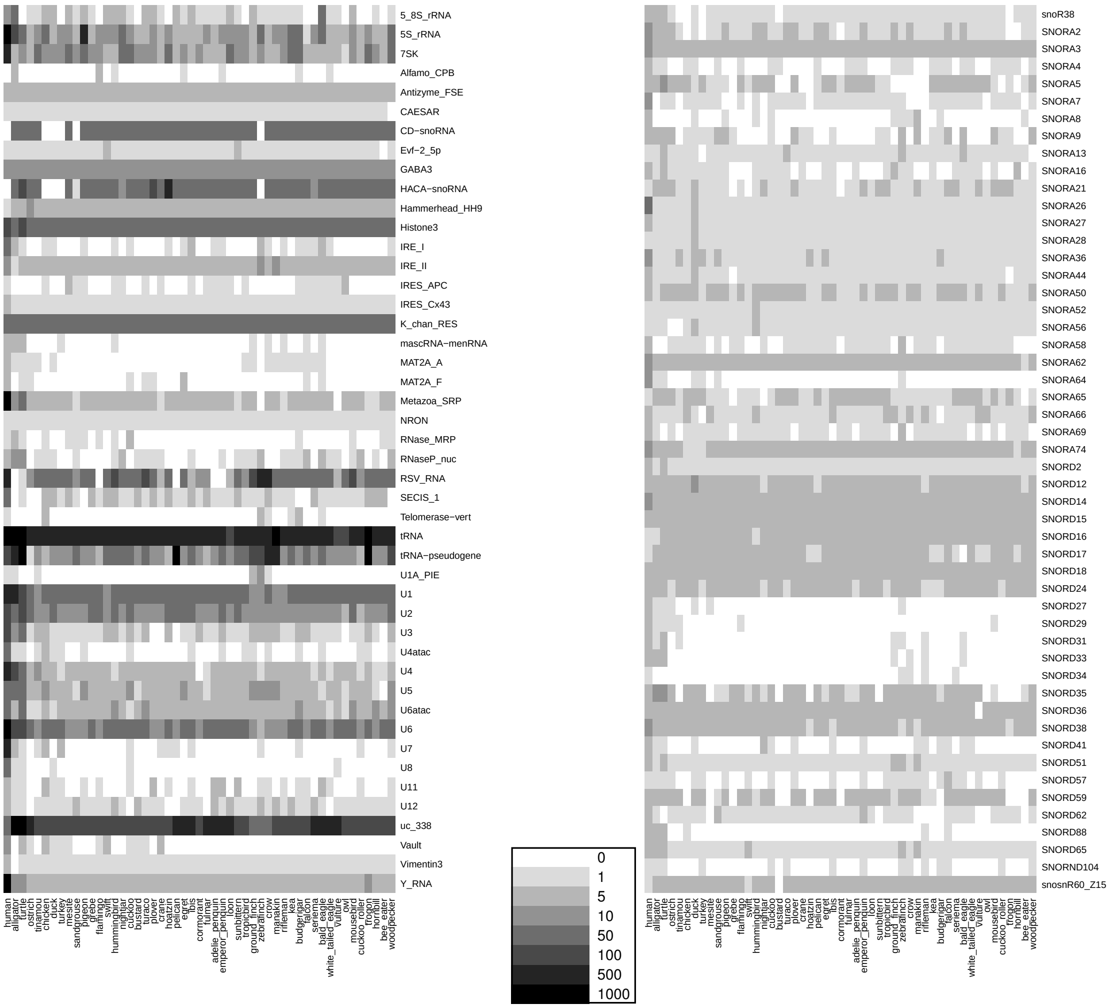

Figure 2: This figure illustrates the number of copies of Rfam and tRNAscan annotations for each RNA family in each avian species and outgroups. The families are ordered alphabetically vertically and the species are in phylogenetic order horizontally. Darker shades indicate high copy numbers, lighter shades indicate fewer, white indicates no predictions were made.

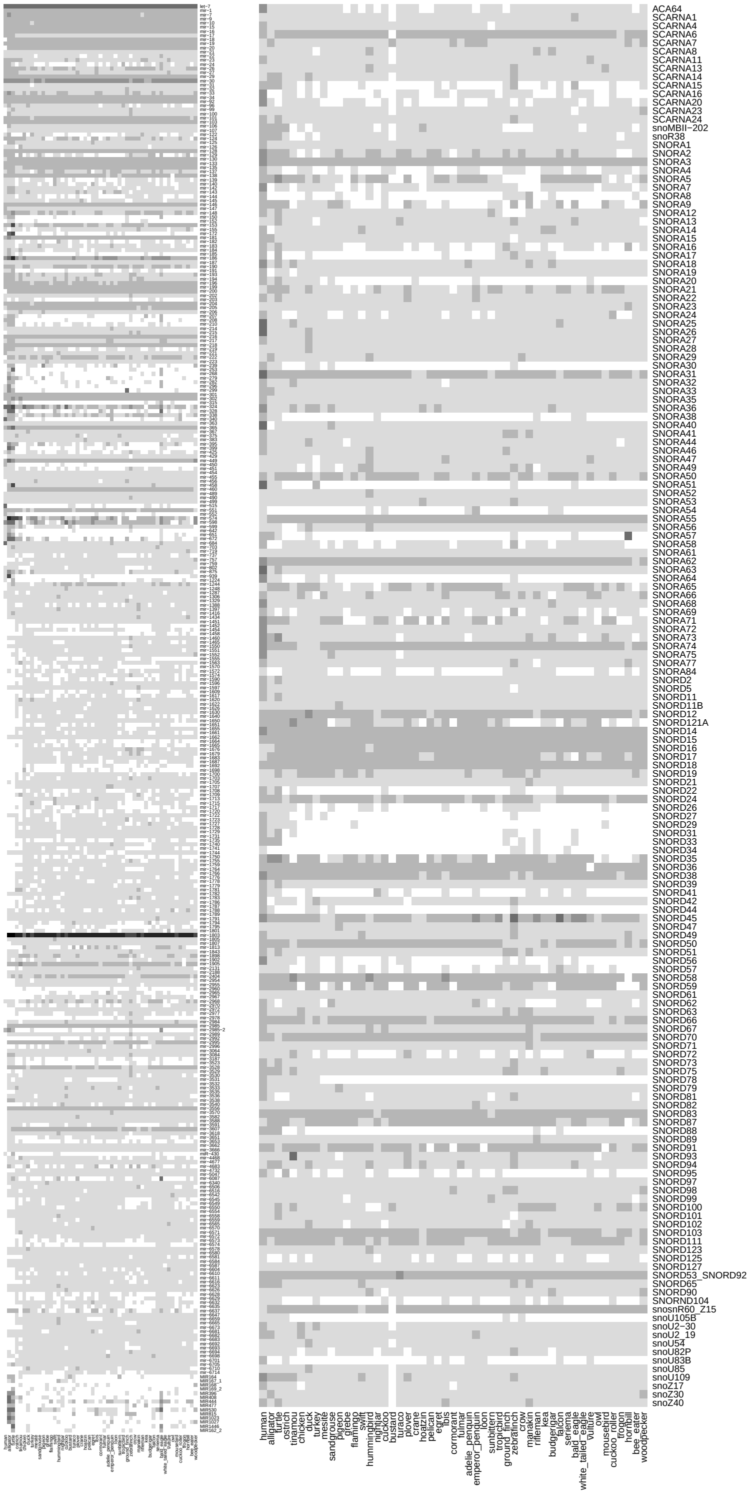

Figure 3: Heatmaps showing the presence/absence and approximate copy number of **miRNA** families on the right and **snoRNA** families on the left.

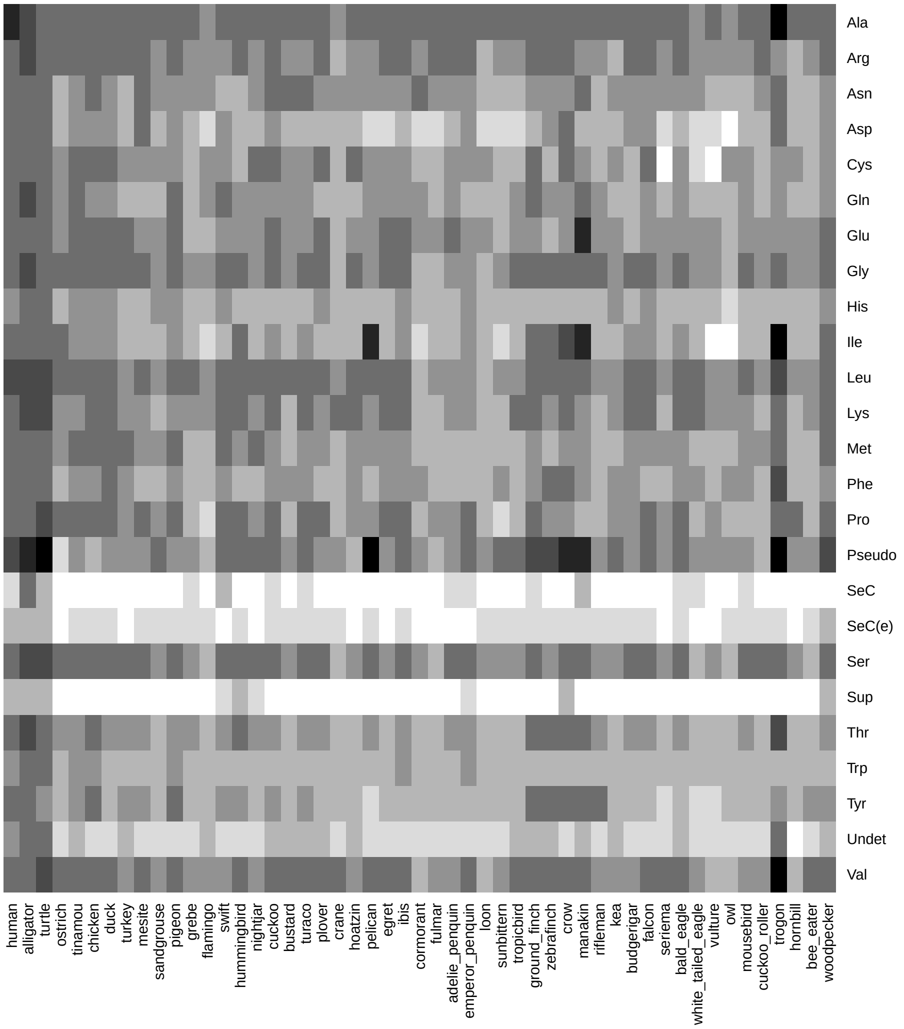


Figure 4: Heatmaps showing the presence/absence and approximate copy number of **tRNA** families.

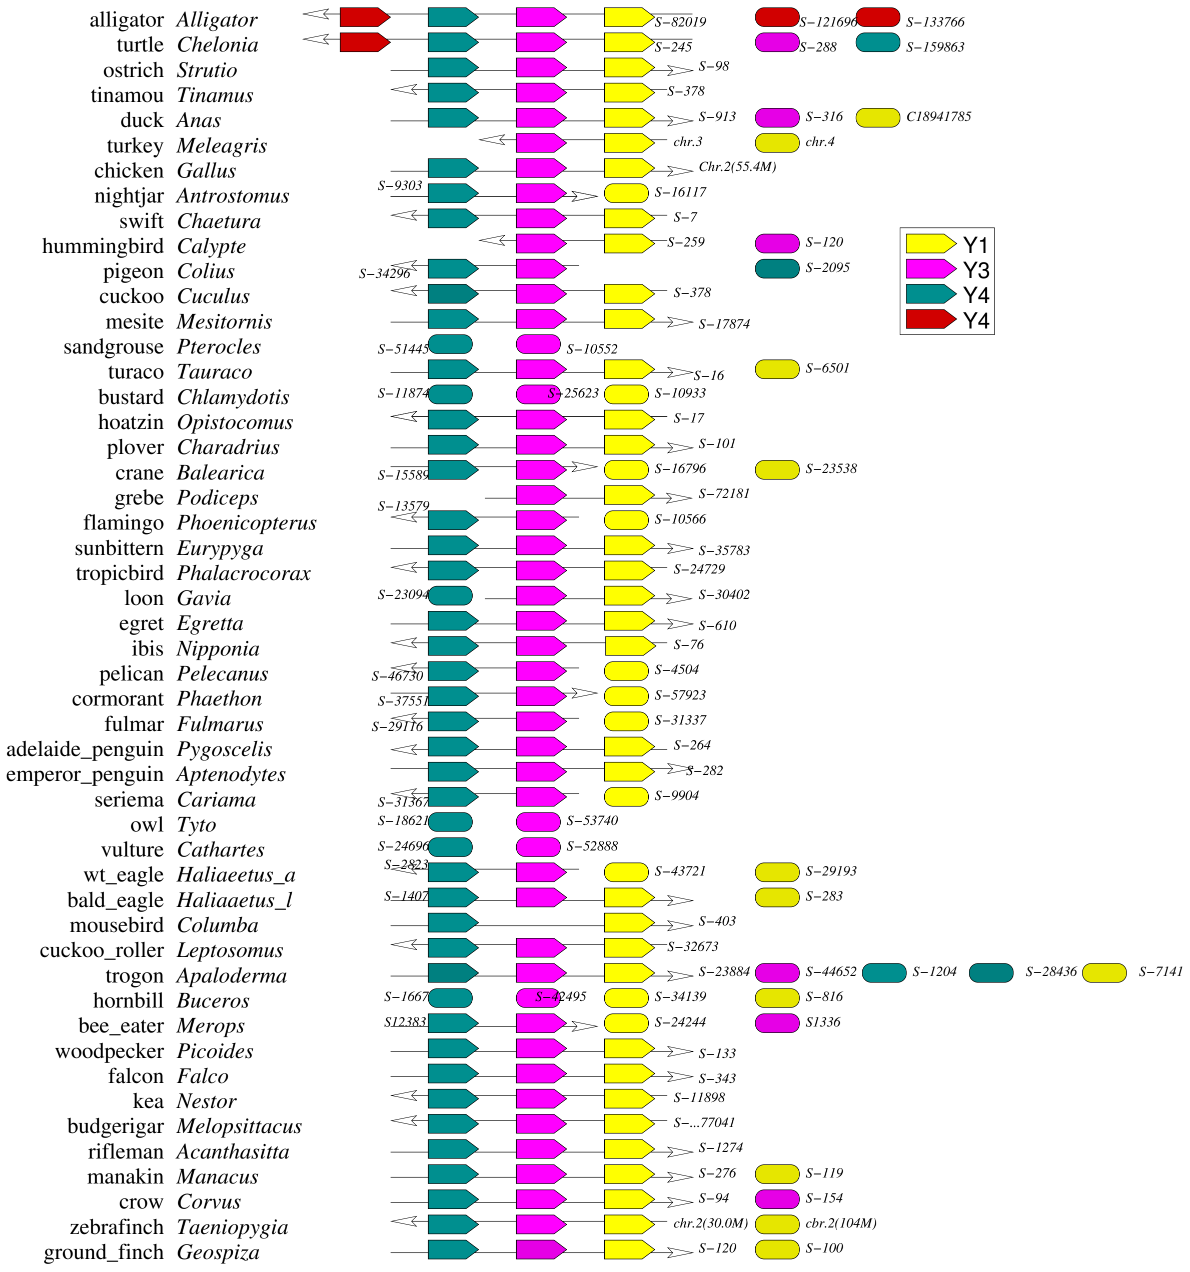


Figure 5: Syntenic conservation of the Y RNA cluster in avian and reptile genomes.

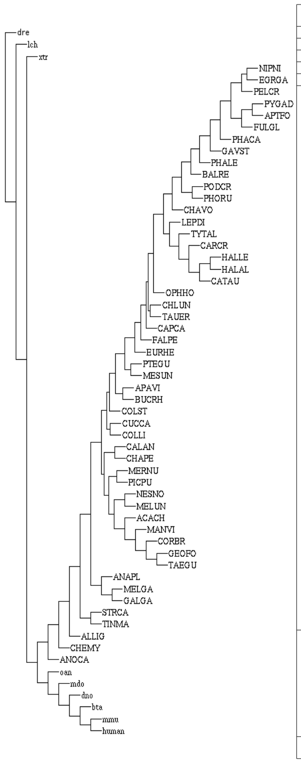


| species | I-1 cluster | | | | | | I-X cluster | | | | | | II | | | |
|---|---|---|---|---|---|---|---|---|---|---|---|---|---|---|---|---|
| | mir-17 | mir-18a | mir-19a | mir-20a | mir-19b-1 | mir-92-1 | mir-106a | mir-18b | mir-20b | mir-19b-2 | mir-92-2 | mir-363 | mir-106b | mir-93 | 19-b-3 | mir-25 |
| **dre** | 1 | 1 | 1 | 1 | 1 | 1 | 1 | 1 | 1 | 1 | 1 | 1 | 0 | 1 | 1 | 1 |
| **lch** | 1 | 1 | 1 | 1 | 1 | 1 | 1 | 1 | 1 | 1 | 1 | 1 | 0 | 1 | 0 | 1 |
| xtr | 1 | 1 | 1 | 1 | 1 | 1 | 1 | 1 | 1 | 1 | 1 | 1 | 0 | 1 | 0 | 1 |
| NIPNI | 1 | 1 | 1 | 1 | 1 | 1 | 1 | 1 | 1 | 1 | 1 | 1 | 0 | 0 | 0 | 0 |
| EGRGA | 1 | 1 | 1 | 1 | 1 | 1 | 1 | 1 | 1 | 1 | 1 | 1 | 0 | 0 | 0 | 0 |
| PELCR | 1 | 1 | 1 | 1 | 1 | 1 | 1 | 1 | 1 | 1 | 1 | 1 | 0 | 0 | 0 | 0 |
| PYGAD | 1 | 1 | 1 | 1 | 1 | 1 | 1 | 1 | 1 | 1 | 1 | 1 | 0 | 0 | 0 | 0 |
| APTFO | 1 | 1 | 1 | 1 | 1 | 1 | 1 | 1 | 1 | 1 | 1 | 1 | 0 | 0 | 0 | 0 |
| FULGL | 1 | 1 | 1 | 1 | 1 | 1 | 1 | 1 | 1 | 1 | 1 | 1 | 0 | 0 | 0 | 0 |
| PHACA | 1 | 1 | 1 | 1 | 1 | 1 | 1 | 1 | 1 | 1 | 1 | 1 | 0 | 0 | 0 | 0 |
| GAVST | 1 | 1 | 1 | 1 | 1 | 1 | 1 | 1 | 1 | 1 | 1 | 1 | 0 | 0 | 0 | 0 |
| PHALE | 1 | 1 | 1 | 1 | 1 | 1 | 1 | 1 | 1 | 1 | 1 | 1 | 0 | 0 | 0 | 0 |
| BALRE | 1 | 1 | 1 | 1 | 1 | 1 | 1 | 1 | 1 | 1 | 1 | 1 | 0 | 0 | 0 | 0 |
| PODCR | 1 | 1 | 1 | 1 | 1 | 1 | 1 | 1 | 1 | 1 | 1 | 1 | 0 | 0 | 0 | 0 |
| PHORU | 1 | 1 | 1 | 1 | 1 | 1 | 1 | 1 | 1 | 1 | 1 | 1 | 0 | 1 | 0 | 0 |
| CHAVO | 1 | 1 | 1 | 1 | 1 | 1 | 1 | 1 | 1 | 1 | 1 | 1 | 0 | 0 | 0 | 0 |
| LEPDI | 1 | 1 | 1 | 1 | 1 | 1 | 1 | 1 | 1 | 1 | 1 | 1 | 0 | 0 | 0 | 0 |
| TYTAL | 1 | 1 | 1 | 1 | 1 | 1 | 1 | 1 | 1 | 1 | 1 | 1 | 0 | 0 | 0 | 0 |
| CARCR | 1 | 1 | 1 | 1 | 1 | 1 | 1 | 1 | 1 | 1 | 1 | 1 | 0 | 0 | 0 | 0 |
| HALLE | 1 | 1 | 1 | 1 | 1 | 1 | 1 | 1 | 1 | 1 | 1 | 1 | 0 | 1 | 0 | 0 |
| HALAL | 1 | 1 | 1 | 1 | 1 | 1 | 1 | 1 | 1 | 1 | 1 | 1 | 0 | 0 | 0 | 0 |
| CATAU | 1 | 1 | 1 | 1 | 1 | 1 | 1 | 1 | 1 | 1 | 1 | 1 | 0 | 0 | 0 | 0 |
| OPIHO | 1 | 1 | 1 | 1 | 1 | 1 | 1 | 1 | 1 | 1 | 1 | 1 | 0 | 0 | 0 | 0 |
| CHLUN | 1 | 1 | 1 | 1 | 1 | 1 | 1 | 1 | 1 | 1 | 1 | 1 | 0 | 0 | 0 | 0 |
| TAUER | 1 | 1 | 1 | 1 | 1 | 1 | 1 | 1 | 1 | 1 | 1 | 1 | 0 | 0 | 0 | 0 |
| ANTCA | 1 | 1 | 1 | 1 | 1 | 1 | 1 | 1 | 1 | 1 | 1 | 1 | 0 | 0 | 0 | 0 |
| FALPE | 1 | 1 | 1 | 1 | 1 | 1 | 1 | 1 | 1 | 1 | 1 | 1 | 0 | 0 | 0 | 0 |
| EURHE | 1 | 1 | 1 | 1 | 1 | 1 | 1 | 1 | 1 | 1 | 1 | 1 | 0 | 0 | 0 | 0 |
| PTEGU | 1 | 1 | 1 | 1 | 1 | 1 | 1 | 1 | 1 | 1 | 1 | 1 | 0 | 0 | 0 | 0 |
| MESUN | 1 | 1 | 1 | 1 | 1 | 1 | 1 | 1 | 1 | 1 | 1 | 1 | 0 | 0 | 0 | 0 |
| APAVI | 1 | 1 | 1 | 1 | 1 | 1 | 1 | 1 | 1 | 1 | 1 | 1 | 0 | 0 | 0 | 0 |
| BUCRH | 1 | 1 | 1 | 1 | 1 | 1 | 1 | 1 | 1 | 1 | 1 | 1 | 0 | 0 | 0 | 0 |
| COLST | 1 | 1 | 1 | 1 | 1 | 1 | 1 | 1 | 1 | 1 | 1 | 1 | 0 | 0 | 0 | 0 |
| CUCCA | 1 | 1 | 1 | 1 | 1 | 1 | 1 | 1 | 1 | 1 | 1 | 1 | 0 | 0 | 0 | 0 |
| COLLI | 1 | 1 | 1 | 1 | 1 | 1 | 1 | 1 | 1 | 1 | 1 | 1 | 0 | 0 | 0 | 0 |
| CALAN | 1 | 1 | 1 | 1 | 1 | 1 | 1 | 1 | 1 | 1 | 1 | 1 | 0 | 0 | 0 | 0 |
| CHAPE | 1 | 1 | 1 | 1 | 1 | 1 | 1 | 1 | 1 | 1 | 1 | 1 | 0 | 0 | 0 | 0 |
| MERNU | 1 | 1 | 1 | 1 | 1 | 1 | 1 | 1 | 1 | 1 | 1 | 1 | 0 | 0 | 0 | 0 |
| PICPU | 1 | 1 | 1 | 1 | 1 | 1 | 1 | 1 | 1 | 1 | 1 | 1 | 0 | 0 | 0 | 0 |
| NESNO | 1 | 1 | 1 | 1 | 1 | 1 | 1 | 1 | 1 | 1 | 1 | 1 | 0 | 0 | 0 | 0 |
| MELUN | 1 | 1 | 1 | 1 | 1 | 1 | 1 | 1 | 1 | 1 | 1 | 1 | 0 | 0 | 0 | 0 |
| ACACH | 1 | 1 | 1 | 1 | 1 | 1 | 1 | 1 | 1 | 1 | 1 | 1 | 0 | 0 | 0 | 0 |
| MANVI | 1 | 1 | 1 | 1 | 1 | 1 | 1 | 1 | 1 | 1 | 1 | 1 | 0 | 0 | 0 | 0 |
| CORBR | 1 | 1 | 1 | 1 | 1 | 1 | 1 | 1 | 1 | 1 | 1 | 1 | 0 | 0 | 0 | 0 |
| GEOFO | 1 | 1 | 1 | 1 | 1 | 1 | 1 | 1 | 1 | 1 | 1 | 1 | 0 | 0 | 0 | 0 |
| TAEGU | 1 | 1 | 1 | 1 | 1 | 1 | 1 | 1 | 1 | 1 | 1 | 1 | 0 | 0 | 0 | 0 |
| ANAPL | 1 | 1 | 1 | 1 | 1 | 1 | 1 | 1 | 1 | 1 | 1 | 1 | 0 | 0 | 0 | 0 |
| MELGA | 1 | 1 | 1 | 1 | 1 | 1 | 1 | 1 | 1 | 1 | 1 | 1 | 0 | 0 | 0 | 0 |
| GALGA | 1 | 1 | 1 | 1 | 1 | 1 | 1 | 1 | 1 | 1 | 1 | 1 | 0 | 0 | 0 | 0 |
| STRCA | 1 | 1 | 1 | 1 | 1 | 1 | 1 | 1 | 1 | 1 | 1 | 1 | 0 | 0 | 0 | 0 |
| TINMA | 1 | 1 | 1 | 1 | 1 | 1 | 1 | 1 | 1 | 1 | 1 | 1 | 0 | 0 | 0 | 0 |
| ALLIG | 1 | 1 | 1 | 1 | 1 | 1 | 1 | 1 | 1 | 1 | 1 | 2 | 1 | 1 | 0 | 0 |
| CHEMY | 1 | 1 | 1 | 1 | 1 | 1 | 1 | 1 | 1 | 1 | 1 | 1 | 0 | 0 | 0 | 0 |
| ANOCA | 1 | 1 | 1 | 1 | 1 | 1 | 1 | 1 | 1 | 1 | 1 | 1 | 0 | 0 | 0 | 0 |
| oan | 2 | 1 | 1 | 1 | 1 | 1 | 1 | 1 | 1 | 1 | 1 | 1 | 0 | 0 | 0 | 0 |
| mdo | 1 | 1 | 1 | 1 | 1 | 1 | 1 | 1 | 1 | 1 | 1 | 1 | 0 | 1 | 0 | 1 |
| dno | 1 | 1 | 1 | 1 | 1 | 1 | 1 | 0 | 0 | 0 | 0 | 0 | 1 | 1 | 0 | 1 |
| bta | 1 | 1 | 1 | 1 | 1 | 1 | 1 | 1 | 1 | 1 | 1 | 1 | 1 | 1 | 0 | 1 |
| mmu | 1 | 1 | 1 | 1 | 1 | 1 | 1 | 1 | 1 | 1 | 1 | 1 | 1 | 1 | 0 | 1 |
| HUMAN | 1 | 1 | 1 | 1 | 1 | 1 | 1 | 1 | 1 | 1 | 1 | 1 | 1 | 1 | 0 | 1 |
| species | mir-17 | mir-18a | mir-19a | mir-20a | mir-19b-1 | mr-92-1 | mir-106a | mir-18b | mir-20b | mir-19b-2 | mir-92-2 | | mir-106b | mir-93 | 19-b-3 | mir-25 |
| | I-1 cluster | | | | | | I-X cluster | | | | | | II | | | |

Figure 6: This figure illustrates the distribution of all members of the mir-17 clusters across birds, compared to fish and mammals. Columns correspond to single miRNA sequences, grouped by clusters and ordered by their position within the corresponding cluster. Rows correspond to the species and the cells contain the number of copies of the miRNA in the respective species. Colors correspond to orthologous miRNA families: mir-17 (orange), mir-19 (blue) and mir-92/25 (green).There are 3 clusters, I-1 and I-X, and cluster II. While the two copies of cluster I are completely conserved, cluster II has been lost as a whole in birds.

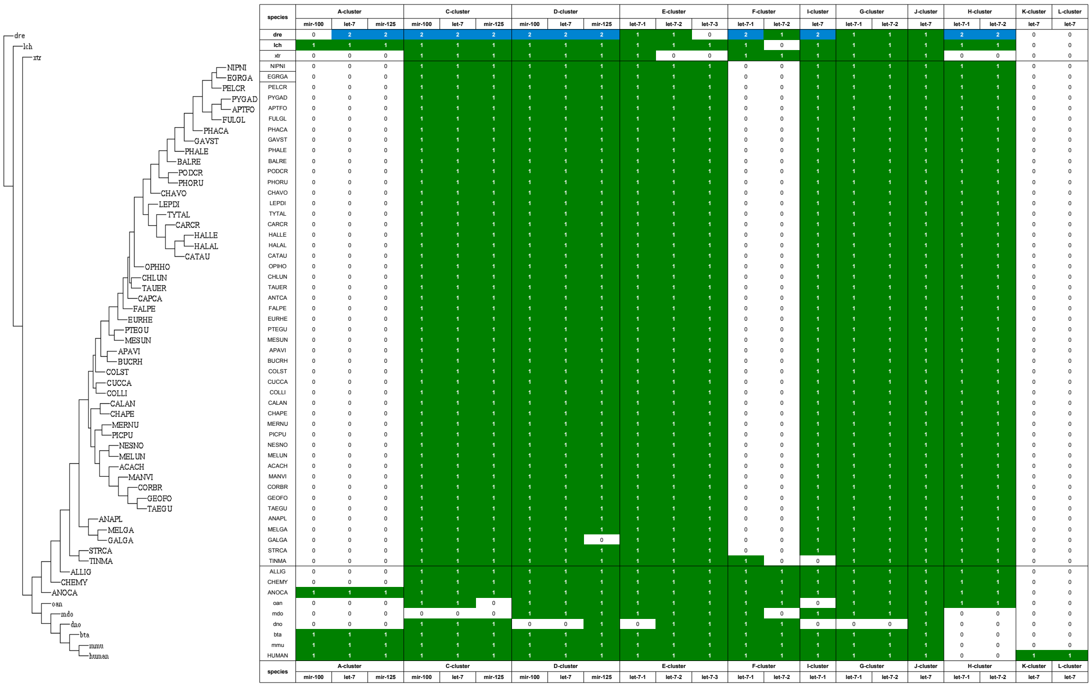

Figure 7: This figure illustrates the distribution of the let-7 paralogs and clustered miRNAs of the families mir-100 and mir-125. Columns correspond to single miRNA sequences, grouped by clusters and ordered by their position within the corresponding cluster. Rows correspond to the species and the cells contain the number of copies of the miRNA in the respective species. Cluster A, which is strongly conserved in vertebrates has been completely lost in the avian lineage. Another obvious loss in birds is cluster F. However, in tinamou we detected an unclustered miRNA that best fits to F-let-7-1 in sequence and structure, while we could not find an I-let-7 miRNA sequence in this species.

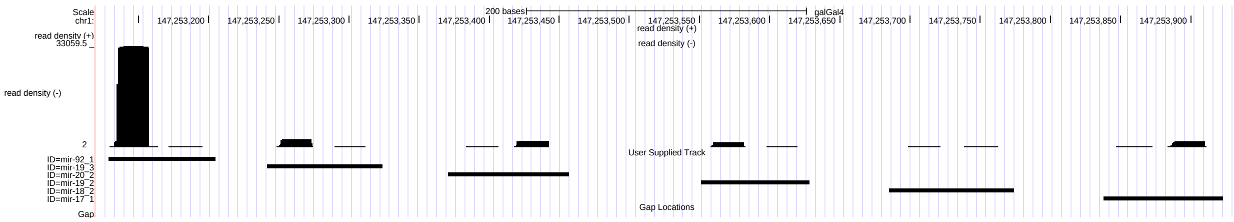


Figure 8: microRNA 17 I-1 cluster: mir-92_1, mir-19_3, mir-20_2, mir-19_2, mir-18_2 & mir-17_1. The figure indicates the genomic location and the RNA-seq read-depths for these 6 microRNAs.

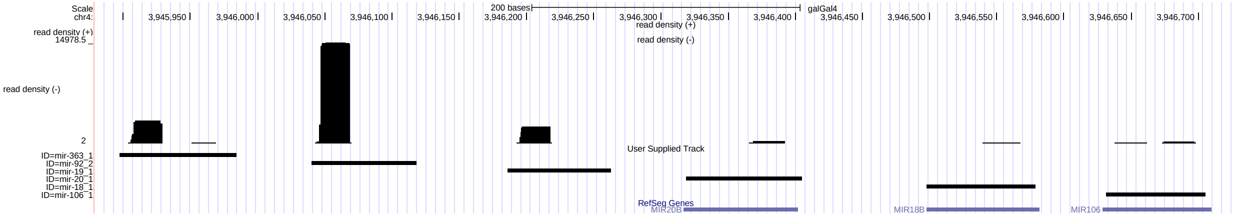


Figure 9: microRNA 17 I-X cluster: mir-363_1, mir-92_2, mir-19_1, mir-20_1, mir-18_1, mir-106_1. The figure indicates the genomic location and the RNA-seq read-depths for these 6 microRNAs.

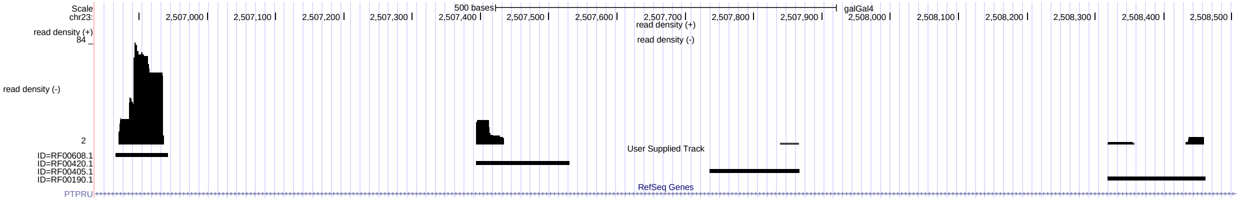


Figure 10: H/ACA box snoRNA cluster: SNORA61, SNORA44, SNORA16. The figure indicates the genomic location and the RNA-seq read-depths for these 3 snoRNAs.

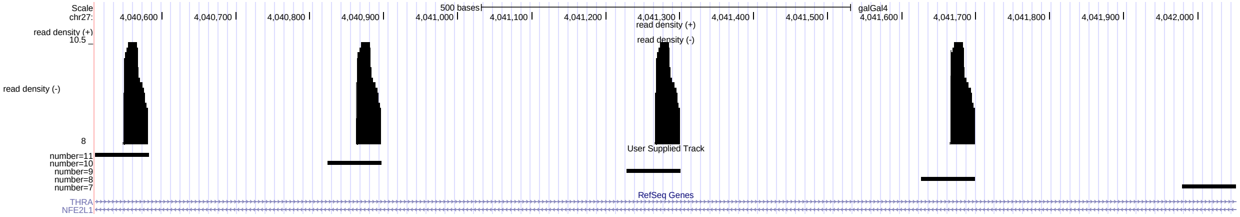


Figure 11: Cysteine tRNA cluster. The figure indicates the genomic location and the RNA-seq read-depths for these 5 transfer RNAs.

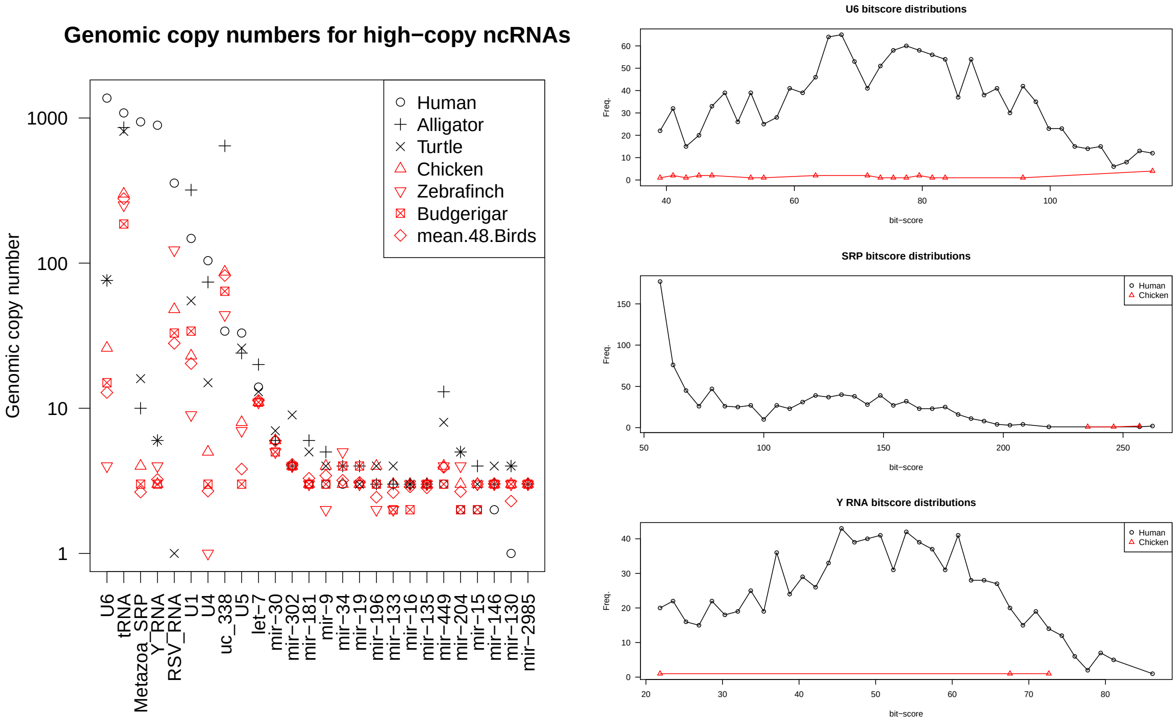


Figure 12: **Left:** A comparison of the genomic copy numbers for 26 of the most abundant RNAs found in human, reptile and the bird genomes. **Right:** Bit-score distributions for the Rfam U6, Metazoan SRP and the Y RNA covariance models for human and chicken paralogues/pseudogenes. Loci with high bit-scores are more likely to be functional than those with low bit-scores (due to excess variation that conflicts with the canonical RNA models).

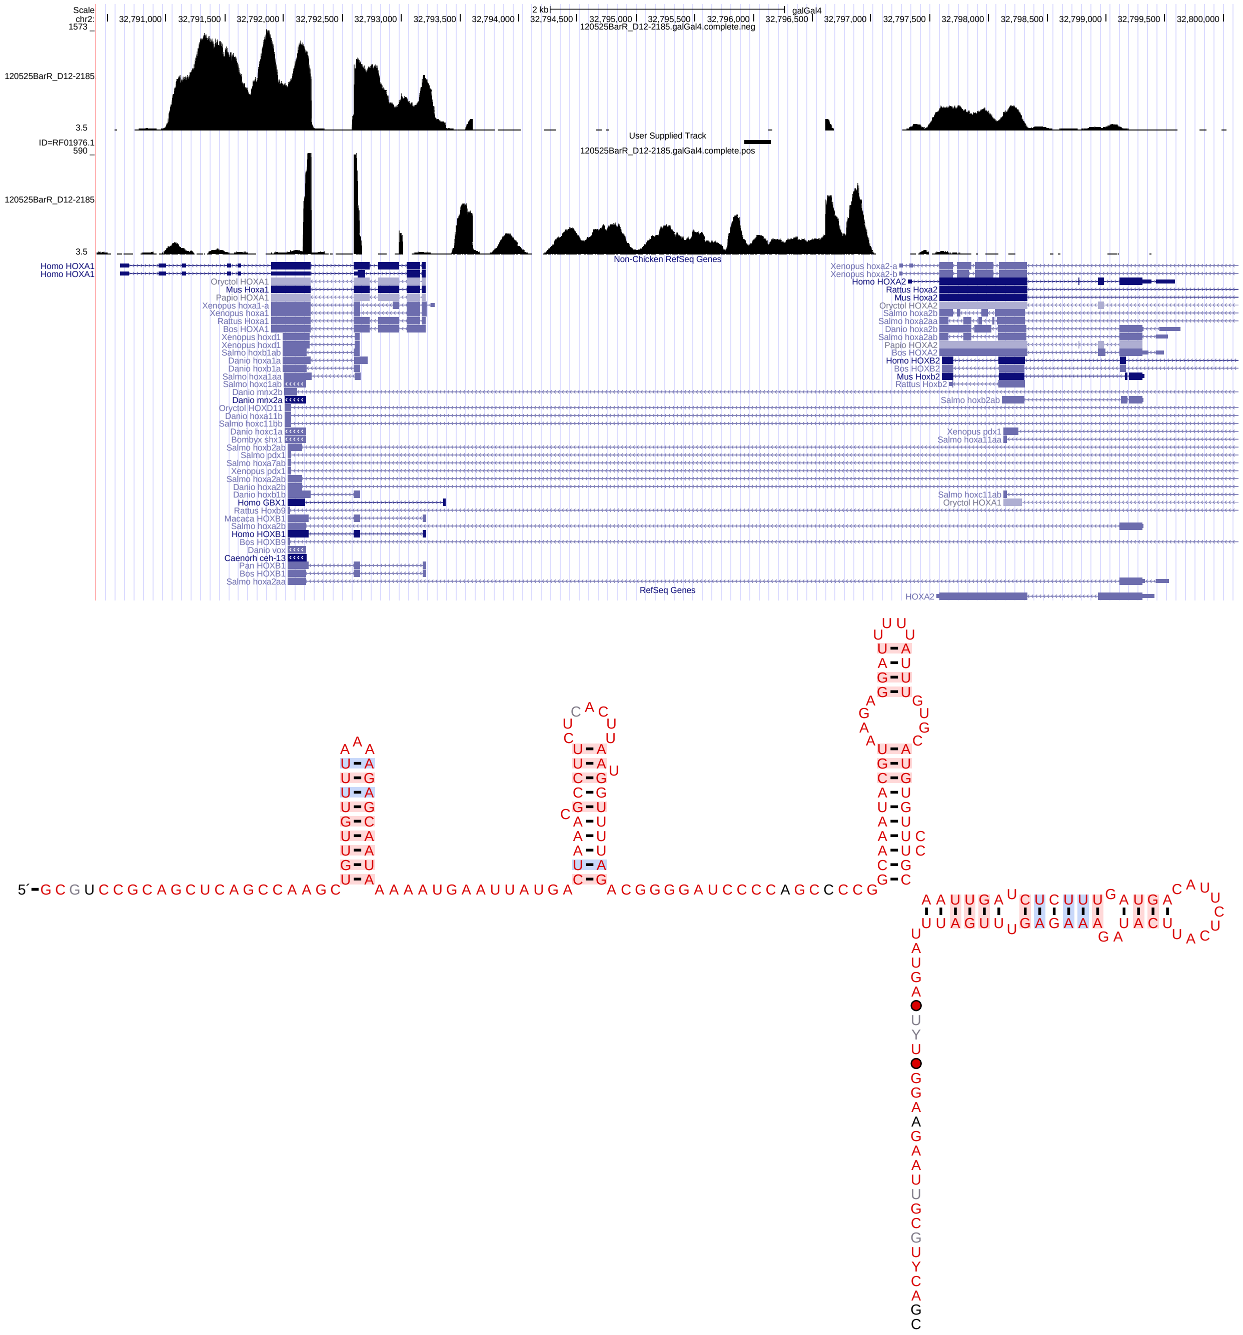

Figure 13: Above: Expression of the chicken HOTAIRM1 (RF01976) locus and the surrounding genes: HOXA1, HOXA2, and HOXA3. Below: The predicted secondary structure of the Avian HOTAIRM1 domain.

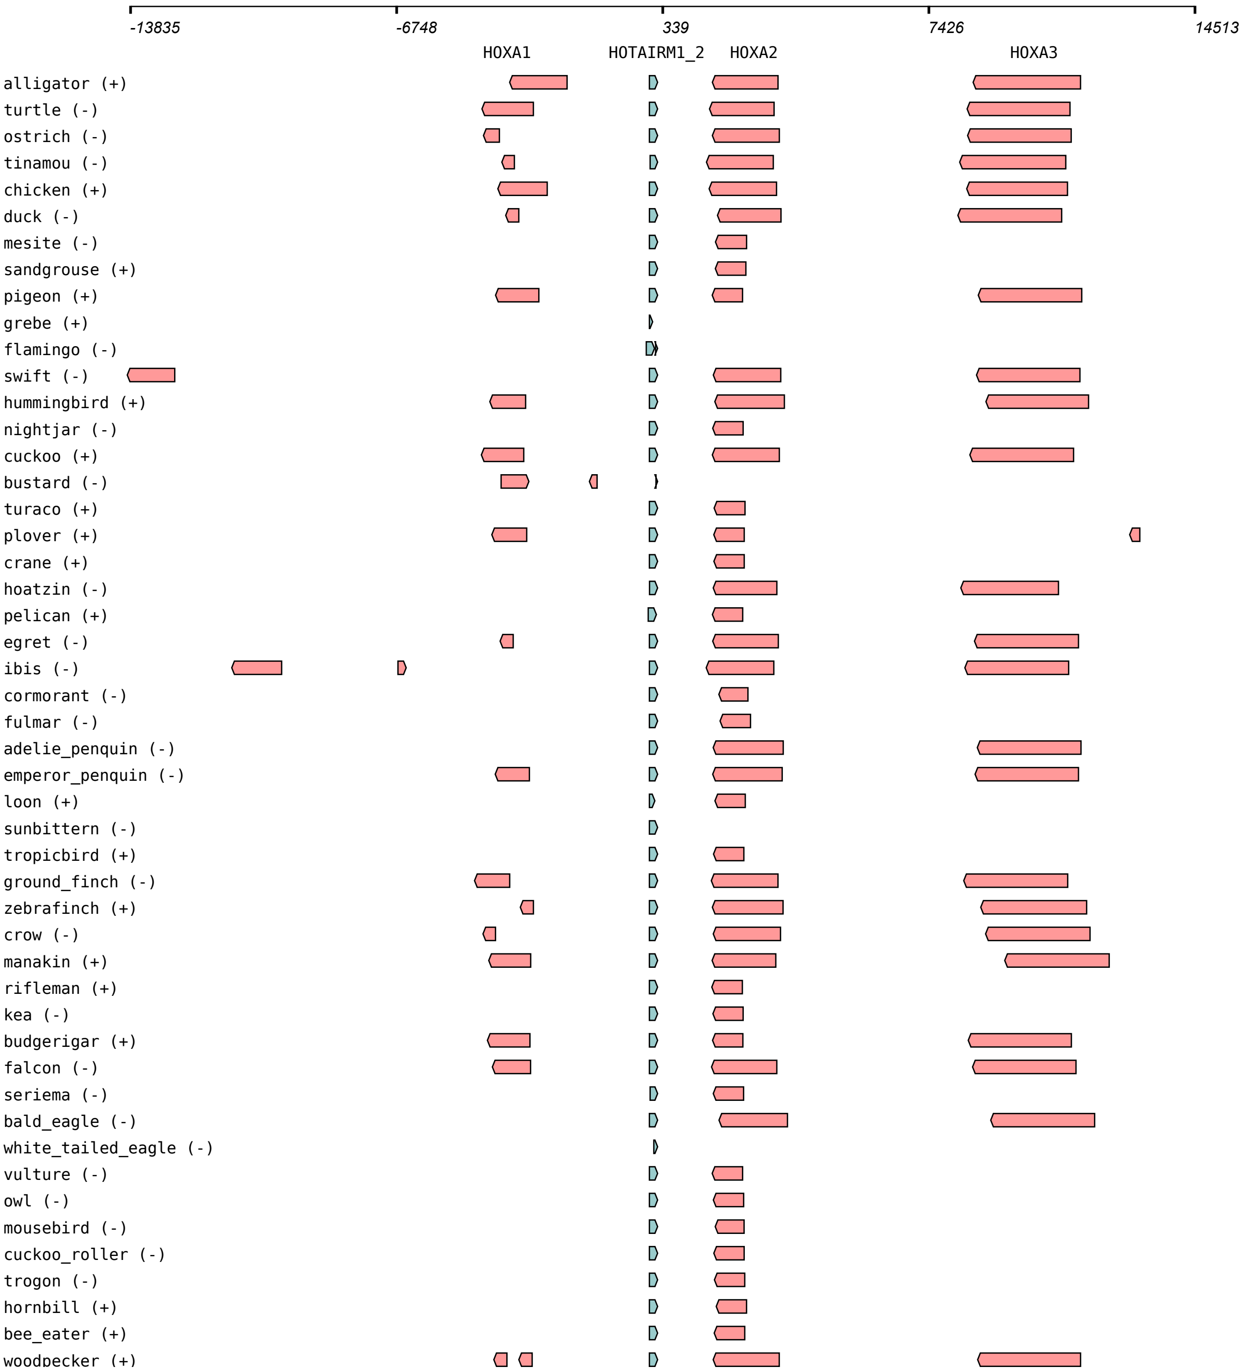


Figure 14: The preservation of gene order (synteny) surrounding the HOTAIRM1 (RF01976) locus across the Avian and other Vertebrate lineages.

| RNA family (Rfam ID) | Chromosome | Coordinates | Strand |
|---|---|---|---|
| **Macro-chromosomes:** | | | |
| RNase MRP (RF00030) | chr4 | 39276202-39276488 | - |
| **Micro-chromosomes:** | | | |
| U4atac snRNA (RF00618) | chr7 | 25702714-25702831 | + |
| RNase P RNA (RF00009) | chr8 | 6609347-6609668 | - |
| Telomerase RNA (RF00024) | chr9 | 19429028-19429084 | + |
| Vault RNA (RF00006) | chr13 | 380747-380840 | + |
| U11 snRNA (RF00548) | chr23 | 2216932-2217058 | - |

Table 1: The location of “missing” RNA families in the chicken genome (galGal4).

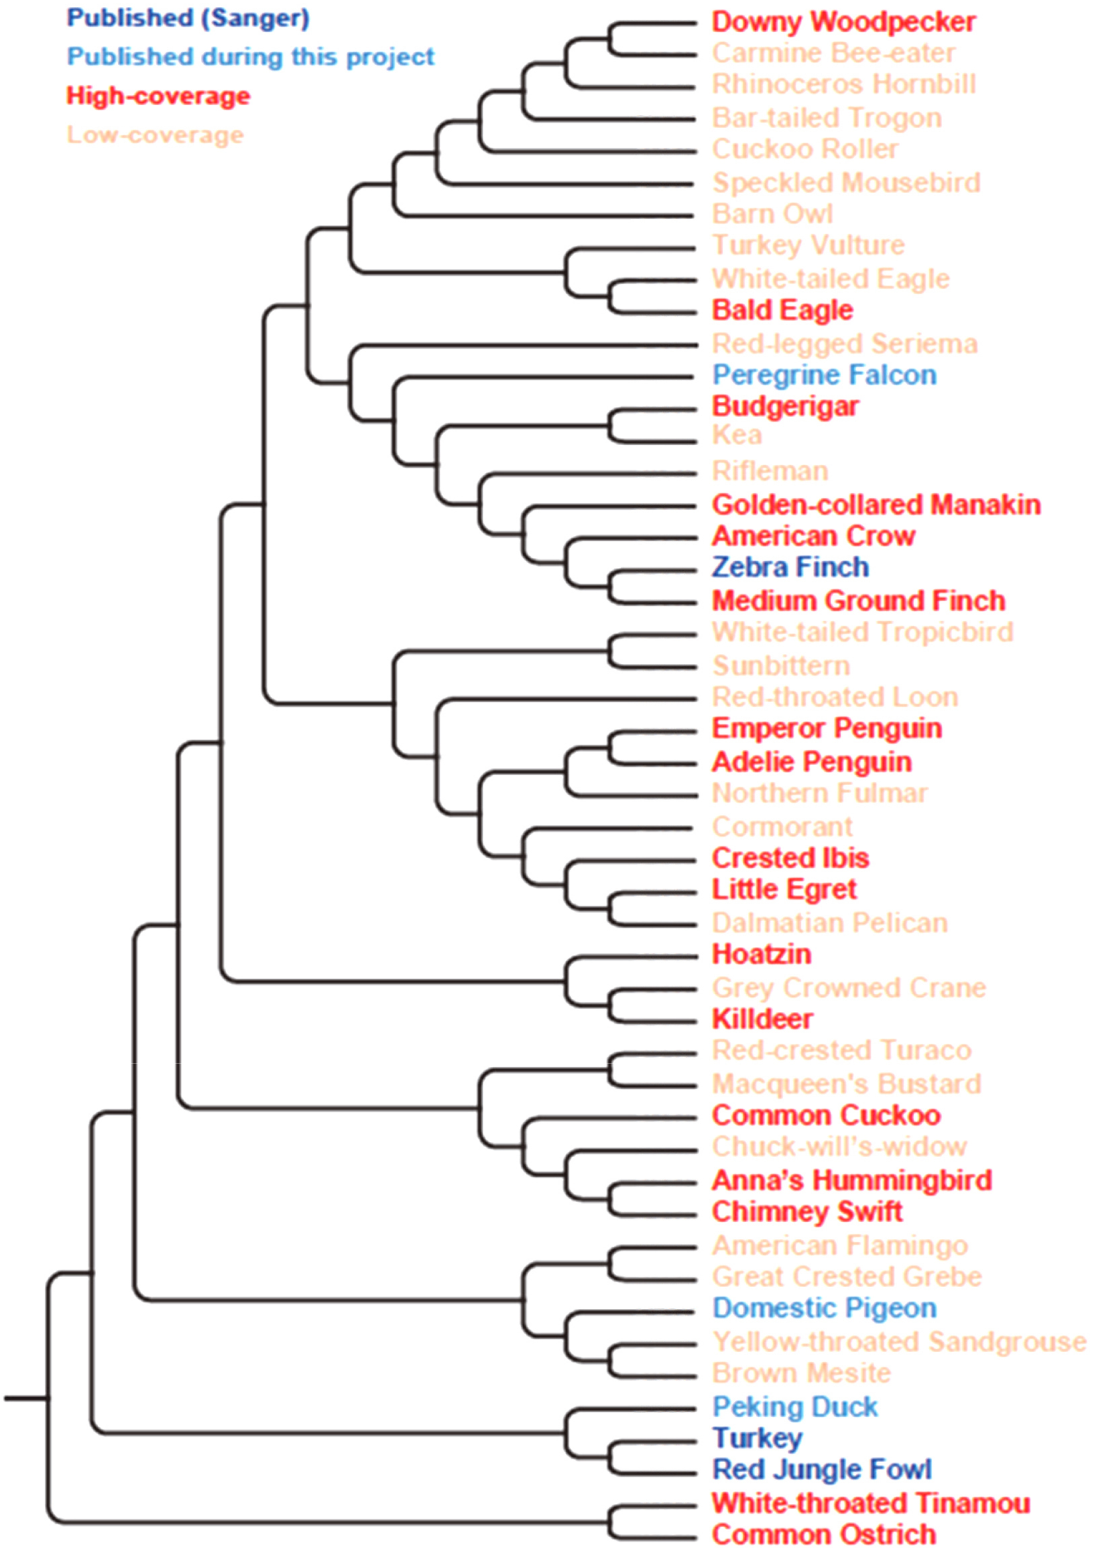


Figure 15: The phylogenetic relationships between the Avian species used in this study. This figure has been reproduced, with permission from [48].

### Database accessions

The NCBI BioProject, SRA and Study IDs for the genomes used in this study are are listed below.

| Name | Species | BioProject ID | SRA ID | Study ID |
|---|---|---|---|---|
| Chimney Swift | *Chaetura pelagica* | PRJNA210808 | SRA092327 | SRP026688 |
| Hummingbird | *Calypte anna* | PRJNA212866 | SRA096094 | SRP028275 |
| Plover | *Charadrius vociferus* | PRJNA212867 | SRA096158 | SRP028286 |
| Crow | *Corvus brachyrhynchos* | PRJNA212869 | SRA096200 | SRP028317 |
| Cuckoo | *Cuculus canorus* | PRJNA212870 | SRA096365 | SRP028349 |
| Manakin | *Manacus vitellinus* | PRJNA212872 | SRA096507 | SRP028393 |
| Hoatzin | *Ophisthocomus hoazin* | PRJNA212873 | SRA096539 | SRP028409 |
| Woodpecker | *Picoides pubescens* | PRJNA212874 | SRA097131 | SRP028625 |
| Ostrich | *Struthio camelus* | PRJNA212875 | SRA097407 | SRP028745 |
| Tinamou | *Tinamus guttatus* | PRJNA212876 | SRA097796 | SRP028753 |
| Rifleman | *Acanthisitta chloris* | PRJNA212877 | SRA097960 | SRP028832 |
| Trogon | *Apaloderma vittatum* | PRJNA212878 | SRA097967 | SRP028834 |
| Crane | *Balearica regulorum* | PRJNA212879 | SRA097970 | SRP028839 |
| Rhinoceros Hornbill | *Buceros rhinoceros* | PRJNA212887 | SRA097991 | SRP028845 |
| Nightjar | *Antrostomus carolinensis* | PRJNA212888 | SRA098079 | SRP028883 |
| Seriema | *Cariama cristata* | PRJNA212889 | SRA098089 | SRP028884 |
| Turkey Vulture | *Cathartes aura* | PRJNA212890 | SRA098145 | SRP028913 |
| Bustard | *Chlamydotis macqueenii* | PRJNA212891 | SRA098203 | SRP028950 |
| Mousebird | *Colius striatus* | PRJNA212892 | SRA098342 | SRP028965 |
| Sunbittern | *Eurypyga helias* | PRJNA212893 | SRA098749 | SRP029147 |
| Northern Fulmar | *Fulmarus glacialis* | PRJNA212894 | SRA098806 | SRP029180 |
| Red-throated Loon | *Gavia stellata* | PRJNA212895 | SRA098829 | SRP029187 |
| White-tailed Eagle | *Haliaeetus albicilla* | PRJNA212896 | SRA098868 | SRP029203 |
| Bald Eagle | *Haliaeetus leucocephalus* | PRJNA237821 | SRX475899 | SRP038924 |
| | | SRX475900 | | |
| | | SRX475901 | | |
| | | SRX475902 | | |
| Cuckoo Roller | *Leptosomus discolor* | PRJNA212897 | SRA098894 | SRP029206 |
| Bee-eater | *Merops nubicus* | PRJNA212898 | SRA099305 | SRP029278 |
| Brown Mesite | *Mesitornis unicolor* | PRJNA212899 | SRA099409 | SRP029309 |
| Kea | *Nestor notabilis* | PRJNA212900 | SRA099410 | SRP029311 |
| Pelican | *Pelecanus crispus* | PRJNA212901 | SRA099411 | SRP029331 |
| Tropicbird | *Phaethon lepturus* | PRJNA212902 | SRA099412 | SRP029342 |
| Cormorant | *Phalacrocorax carbo* | PRJNA212903 | SRA099413 | SRP029344 |
| Flamingo | *Phoenicopterus ruber* | PRJNA212904 | SRA099414 | SRP029345 |
| Grebe | *Podiceps cristatus* | PRJNA212905 | SRA099415 | SRP029346 |
| Sandgrouse | *Pterocles gutturalis* | PRJNA212906 | SRA099416 | SRP029347 |
| Turaco | *Tauraco erythrolophus* | PRJNA212908 | SRA099418 | SRP029348 |
| Barn Owl | *Tyto alba* | PRJNA212909 | SRA099419 | SRP029349 |
| Crested Ibis | *Nipponia nippon* | PRJNA232572 | SRA122361 | SRP035852 |
| Little Egret | *Egretta garzetta* | PRJNA232959 | SRA123137 | SRP035853 |

Table 2: The NCBI BioProject/SRA and Study IDs used in this study.

| Species | BioProject ID | SRA ID | Study ID | |
|---|---|---|---|---|
| Emperor Penguin | *Aptenodytes forsteri* | PRJNA235982 | SRA129317 | SRP035855 |
| Adelie Penguin | *Pygoscelis adeliae* | PRJNA235983 | SRA129318 | SRP035856 |
| Chicken | *Gallus gallus* | PRJNA13342 | SRA030184 | SRP005856 (galGal4) |
| Zebra Finch | *Taeniopygia guttata* | PRJNA17289 | SRA010067 | SRP001389 |
| Turkey | *Meleagris gallopavo* | PRJNA42129 | Unknown | Unknown |
| Budgerigar | *Melopsittacus undulatus* | PRJEB1588 | ERA200248 | ERP002324 |
| Mallard | *Anas platyrhynchos* | PRJNA46621 | SRA010308 | SRP001571 |
| Rock Pigeon | *Columba livia* | PRJNA167554 | SRA054954 | SRP013894 |
| Peregrine Falcon | *Falco peregrinus* | PRJNA159791 | SRA055082 | SRP013939 |
| Medium Ground-finch | *Geospiza fortis* | PRJNA156703 | SRA051234 | SRP011940 |
| Outgroups | | | | |
| Human | *Homo sapiens* | | | HG19/GRCh37 |
| Alligator | *Alligator mississippiensis* | | | allMis1 |
| Green Turtle | *Chelonia mydas* | PRJNA104937 | | |
| RNA-seq data | | | | |
| Chicken | *Gallus gallus* | PRJNA204941 | NA | NA |
| Chicken | *Gallus gallus* | NA | NA | SRP041863 |

Table 3: The NCBI BioProject/SRA and Study IDs for the previously published genomes used in this study.

## References


1. Jeffares DC, Poole AM, Penny D: **Relics from the RNA world.** *J Mol Evol* 1998, **46**:18–36.
2. Hoeppner MP, Gardner PP, Poole AM: **Comparative analysis of RNA families reveals distinct repertoires for each domain of life.** *PLoS Comput Biol* 2012, **8**(11):e1002752.
3. Leonardi J, Box JA, Bunch JT, Baumann P: **TER1, the RNA subunit of fission yeast telomerase.** *Nat Struct Mol Biol* 2008, **15**:26–33.
4. Webb CJ, Zakian VA: **Identification and characterization of the Schizosaccharomyces pombe TER1 telomerase RNA.** *Nat Struct Mol Biol* 2008, **15**:34–42.
5. Mao C, Bhardwaj K, Sharkady SM, Fish RI, Driscoll T, Wower J, Zwieb C, Sobral BW, Williams KP: **Variations on the tmRNA gene.** *RNA Biol* 2009, **6**(4):355–61.
6. Lai LB, Chan PP, Cozen AE, Bernick DL, Brown JW, Gopalan V, Lowe TM: **Discovery of a minimal form of RNase P in Pyrobaculum.** *Proc Natl Acad Sci U S A* 2010, **107**(52):22493–8.
7. Chan PP, Cozen AE, Lowe TM: **Discovery of permuted and recently split transfer RNAs in Archaea.** *Genome Biol* 2011, **12**(4):R38.
8. Dávila López M, Rosenblad MA, Samuelsson T: **Computational screen for spliceosomal RNA genes aids in defining the phylogenetic distribution of major and minor spliceosomal components.** *Nucleic Acids Res* 2008, **36**(9):3001–10.
9. Marz M, Kirsten T, Stadler PF: **Evolution of spliceosomal snRNA genes in metazoan animals.** *J Mol Evol* 2008, **67**(6):594–607.
10. López MD, Rosenblad MA, Samuelsson T: **Conserved and variable domains of RNase MRP RNA.** *RNA Biol* 2009, **6**(3).
11. Rosenblad MA, López MD, Piccinelli P, Samuelsson T: **Inventory and analysis of the protein subunits of the ribonucleases P and MRP provides further evidence of homology between the yeast and human enzymes.** *Nucleic Acids Res* 2006, **34**(18):5145–56.
12. Floutsakou *et al*: **The shared genomic architecture of human nucleolar organizer regions**. *Genome Research* 2013.
13. Gardner PP, Bateman A, Poole AM: **SnoPatrol: how many snoRNA genes are there?** *J Biol* 2010, **9**:4.

14. Marz M, Gruber AR, Höner Zu Siederdissen C, Amman F, Badelt S, Bartschat S, Bernhart SH, Beyer W, Kehr S, Lorenz R, Tanzer A, Yusuf D, Tafer H, Hofacker IL, Stadler PF: **Animal snoRNAs and scaRNAs with exceptional structures.** *RNA Biol* 2011, **8**(6).

15. Lestrade L, Weber MJ: **snoRNA-LBME-db, a comprehensive database of human H/ACA and C/D box snoRNAs.** *Nucleic Acids Res* 2006, **34**(Database issue):D158–62.

16. Tycowski KT, Shu MD, Steitz JA: **A mammalian gene with introns instead of exons generating stable RNA products.** *Nature* 1996, **379**(6564):464–6.

17. Cock JM, Sterck L, Rouzé P, Scornet D, Allen AE, Amoutzias G, Anthouard V, Artiguenave F, Aury JM, Badger JH, Beszteri B, Billiau K, Bonnet E, Bothwell JH, Bowler C, Boyen C, Brownlee C, Carrano CJ, Charrier B, Cho GY, Coelho SM, Collén J, Corre E, Da Silva C, Delage L, Delaroque N, Dittami SM, Doulbeau S, Elias M, Farnham G, Gachon CM, Gschloessl B, Heesch S, Jabbari K, Jubin C, Kawai H, Kimura K, Kloareg B, Küpper FC, Lang D, Le Bail A, Leblanc C, Lerouge P, Lohr M, Lopez PJ, Martens C, Maumus F, Michel G, Miranda-Saavedra D, Morales J, Moreau H, Motomura T, Nagasato C, Napoli CA, Nelson DR, Nyvall-Collén P, Peters AF, Pommier C, Potin P, Poulain J, Quesneville H, Read B, Rensing SA, Ritter A, Rousvoal S, Samanta M, Samson G, Schroeder DC, Ségurens B, Strittmatter M, Tonon T, Tregear JW, Valentin K, von Dassow P, Yamagishi T, Van de Peer Y, Wincker P: **The Ectocarpus genome and the independent evolution of multicellularity in brown algae.** *Nature* 2010, **465**(7298):617–21.

18. Huang A, He L, Wang G: **Identification and characterization of microRNAs from Phaeodactylum tricornutum by high-throughput sequencing and bioinformatics analysis.** *BMC Genomics* 2011, **12**:337.

19. Lee RC, Feinbaum RL, Ambros V: **The C. elegans heterochronic gene lin-4 encodes small RNAs with antisense complementarity to lin-14.** *Cell* 1993, **75**(5):843–54.

20. Lau NC, Lim LP, Weinstein EG, Bartel DP: **An abundant class of tiny RNAs with probable regulatory roles in Caenorhabditis elegans.** *Science* 2001, **294**(5543):858–62.

21. Hertel J, Lindemeyer M, Missal K, Fried C, Tanzer A, Flamm C, Hofacker IL, Stadler PF, of Bioinformatics Computer Labs 2004 S, 2005 C: **The expansion of the metazoan microRNA repertoire.** *BMC Genomics* 2006, **7**:25.

22. Hinas A, Reimegård J, Wagner EG, Nellen W, Ambros VR, Söderbom F: **The small RNA repertoire of Dictyostelium discoideum and its regulation by components of the RNAi pathway.** *Nucleic Acids Res* 2007, **35**(20):6714–26.

23. Avesson L, Reimegård J, Wagner EG, Söderbom F: **MicroRNAs in Amoebozoa: deep sequencing of the small RNA population in the social amoeba Dictyostelium discoideum reveals developmentally regulated microRNAs.** *RNA* 2012, **18**(10):1771–82.

24. Reinhart BJ, Weinstein EG, Rhoades MW, Bartel B, Bartel DP: **MicroRNAs in plants.** *Genes Dev* 2002, **16**(13):1616–26.

25. Fattash I, Voss B, Reski R, Hess WR, Frank W: **Evidence for the rapid expansion of microRNA-mediated regulation in early land plant evolution.** *BMC Plant Biol* 2007, **7**:13.

26. Axtell MJ, Snyder JA, Bartel DP: **Common functions for diverse small RNAs of land plants.** *Plant Cell* 2007, **19**(6):1750–69.

27. Molnár A, Schwach F, Studholme DJ, Thuenemann EC, Baulcombe DC: **miRNAs control gene expression in the single-cell alga Chlamydomonas reinhardtii.** *Nature* 2007, **447**(7148):1126–9.

28. Pfeffer S, Zavolan M, Grässer FA, Chien M, Russo JJ, Ju J, John B, Enright AJ, Marks D, Sander C, Tuschl T: **Identification of virus-encoded microRNAs.** *Science* 2004, **304**(5671):734–6.

29. Ouellet DL, Plante I, Landry P, Barat C, Janelle ME, Flamand L, Tremblay MJ, Provost P: **Identification of functional microRNAs released through asymmetrical processing of HIV-1 TAR element.** *Nucleic Acids Res* 2008, **36**(7):2353–65.

30. Pfeffer S, Sewer A, Lagos-Quintana M, Sheridan R, Sander C, Grässer FA, van Dyk LF, Ho CK, Shuman S, Chien M, Russo JJ, Ju J, Randall G, Lindenbach BD, Rice CM, Simon V, Ho DD, Zavolan M, Tuschl T: **Identification of microRNAs of the herpesvirus family.** *Nat Methods* 2005, **2**(4):269–76.

31. Landgraf P, Rusu M, Sheridan R, Sewer A, Iovino N, Aravin A, Pfeffer S, Rice A, Kamphorst AO, Landthaler M, Lin C, Socci ND, Hermida L, Fulci V, Chiaretti S, Foà R, Schliwka J, Fuchs U, Novosel A, Müller RU, Schermer B, Bissels U, Inman J, Phan Q, Chien M, Weir DB, Choksi R, De Vita G, Frezzetti D, Trompeter HI, Hornung V, Teng G, Hartmann G, Palkovits M, Di Lauro R, Wernet P, Macino G, Rogler CE, Nagle JW, Ju J, Papavasiliou FN, Benzing T, Lichter P, Tam W, Brownstein MJ, Bosio A, Borkhardt A, Russo JJ, Sander C, Zavolan M, Tuschl T: **A mammalian microRNA expression atlas based on small RNA library sequencing.** *Cell* 2007, **129**(7):1401–14.

32. Lim LP, Lau NC, Garrett-Engele P, Grimson A, Schelter JM, Castle J, Bartel DP, Linsley PS, Johnson JM: **Microarray analysis shows that some microRNAs downregulate large numbers of target mRNAs.** *Nature* 2005, **433**(7027):769–73.

33. Stevens SG, Gardner PP, Brown C: **Two covariance models for iron-responsive elements.** *RNA Biol***8**(5):792–801.

34. López D, Samuelsson T: **Early evolution of histone mRNA 3' end processing.** *RNA* 2008, **14**:1–10.

35. Lambert A, Lescure A, Gautheret D: **A survey of metazoan selenocysteine insertion sequences.** *Biochimie* 2002, **84**(9):953–9.

36. Ohlson J, Pedersen JS, Haussler D, Ohman M: **Editing modifies the GABA(A) receptor subunit alpha3.** *RNA* 2007, **13**(5):698–703.

37. Xie M, Mosig A, Qi X, Li Y, Stadler PF, Chen JJL: **Size Variation and Structural Conservation of Vertebrate Telomerase RNA**. *J. Biol. Chem.* 2008, **283**:2049–2059.

38. Stadler PF, Chen JJL, Hackermüller J, Hoffmann S, Horn F, Khaitovich P, Kretzschmar AK, Mosig A, Prohaska SJ, Qi X, Schutt K, Ullmann K: **Evolution of Vault RNAs**. *Mol. Biol. Evol.* 2009, **26**:1975–1991.

39. Kolbe DL, Eddy SR: **Local RNA structure alignment with incomplete sequence.** *Bioinformatics* 2009, **25**(10):1236–43.

40. Bejerano G, Pheasant M, Makunin I, Stephen S, Kent WJ, Mattick JS, Haussler D: **Ultraconserved elements in the human genome.** *Science* 2004, **304**(5675):1321–5.

41. Bejerano G, Lowe CB, Ahituv N, King B, Siepel A, Salama SR, Rubin EM, Kent WJ, Haussler D: **A distal enhancer and an ultraconserved exon are derived from a novel retroposon.** *Nature* 2006, **441**(7089):87–90.

42. Braconi C, Valeri N, Kogure T, Gasparini P, Huang N, Nuovo GJ, Terracciano L, Croce CM, Patel T: **Expression and functional role of a transcribed noncoding RNA with an ultraconserved element in hepatocellular carcinoma.** *Proc Natl Acad Sci U S A* 2011, **108**(2):786–91.

43. Lerner MR, Boyle JA, Hardin JA, Steitz JA: **Two novel classes of small ribonucleoproteins detected by antibodies associated with lupus erythematosus.** *Science* 1981, **211**(4480):400–2.

44. Christov CP, Gardiner TJ, Szüts D, Krude T: **Functional requirement of noncoding Y RNAs for human chromosomal DNA replication.** *Mol Cell Biol* 2006, **26**(18):6993–7004.

45. Mosig A, Guofeng M, Stadler BM, Stadler PF: **Evolution of the vertebrate Y RNA cluster.** *Theory Biosci* 2007, **126**:9–14.

46. Kong LB, Siva AC, Rome LH, Stewart PL: **Structure of the vault, a ubiquitous celular component.** *Structure* 1999, **7**(4):371–9.

47. Stadler PF, Chen JJ, Hackermüller J, Hoffmann S, Horn F, Khaitovich P, Kretzschmar AK, Mosig A, Prohaska SJ, Qi X, Schutt K, Ullmann K: **Evolution of vault RNAs.** *Mol Biol Evol* 2009, **26**(9):1975–91.

48. Avian Phylogenomics Consortium: **Using whole genomes to resolve the tree of life of modern birds**. *In press* 2014.
